# Supplementary material for: Truly Unordered Probabilistic Rule Sets for Multi-class Classification
Source: arXiv:2206.08804 source file (2022-07-18)
Supplement: Supplementary file 1 [file supplementary.tex]

\section*{Reproducibility for Experiments}
\paragraph{Decision trees for surrogate score.} We use a CART decision tree~\cite{breiman1984classification} to get the tree-based surrogate score. For efficiency and robustness, we do not use any post-pruning for the decision tree but only set the minimum sample size on leafs, denoted as $s$. Specifically, we try $s \in \{10, 30, 50, 70, 90\}$ and hence calculate five surrogate scores accordingly, among which we pick the smallest as the final surrogate score. 

\paragraph{Beam width and coverage diversity.} 
% Intuitively, the coverage diversity $\alpha$ can be very small (or even 0) if the beam width is large enough. Thus, in practice, 
We set the coverage diversity $\alpha=0.05$, and beam width $w = 5$. With the coverage diversity as a constraint, we found that $w \in \{5, 10, 20\}$ gives similar results. Due to the limited space, we leave formal sensitivity analysis of $\alpha$ as future work. 

\paragraph{Number of cut points for numeric features.}
To generate literals for numeric features, we need to decide the number of cut points for these features. In practice, it should depend on how the analysts want to interpret the resulting rules: given a specific task, is it useful to be more precise than the granularity of the 10- or 20-quantiles? Intuitively, we believe it is seldom necessary to be more precise than $100$-quantiles, and hence we set the number of cut points as $100$. 
\paragraph{Benchmark datasets and competitor algorithms.}
For reproducibility, we use the implementation of CN2 from Orange3~\cite{JMLR:demsar13a}, RIPPER from RWeka~\cite{Rweka2009}, CART from Sklearn~\cite{scikit-learn}, and BRS and DRS from the authors' original implementation. Most parameters are set as ``default" based on the implementation. For BRS and DRS, this means that we use what the author suggested in the original papers. Specifically, for CART, we use the post-pruning for trees with the regularization parameter chosen from cross-validation.

\section*{Proof of Proposition 1}
\begin{proposition}
Given a rule set $\ruleset$ in which for any $S_i, S_j \in \ruleset$, $S_i \cap S_j = \emptyset$, then $P^{NML}_{\ruleset}(Y^n=y^n|X^n=x^n) = P^{apprNML}_{\ruleset}(Y^n=y^n|X^n=x^n)$.
\end{proposition}
\begin{proof}
The numerators are the same, and hence we only need to show that the denominators are the same. Assume there are $K$ rules in $M$ in total, 
\begin{equation} 
\begin{split}
		& \sum_{z^n \in \mathscr{Y}^n} P_{M, \htheta(x^n, z^n)}(z^n|x^n) = \sum_{z^n} \prod_{S\in M} \hat{P}_S(y^S|X^S) \\
		& = \sum_{z^n} \hat{P}_{_{S_1}}(z^{S_1}|x^{S_1}) \ldots \hat{P}_{_{S_K}}(z^{S_{K}}|x^{S_{K}}) \\
		& = \sum_{z^{S_1}} \ldots \sum_{z^{S_{K}}} \left(\hat{P}_{_{S_1}}(z^{S_1}|x^{S_1}) \ldots \hat{P}_{_{S_K}}(z^{S_{K}}|x^{S_{K}}) \right)\\
		& = \Bigg(\sum_{z^{S_1}} \ldots \sum_{z^{S_{K-1}}} \hat{P}_{_{S_1}}(z^{S_1}|x^{S_1}) \ldots \hat{P}_{_{S_{K-1}}} (z^{S_{K-1}}|x^{S_{K-1}}) \Bigg) \left(\sum_{z^{S_{K}}}  \hat{P}_{_{S_K}}(z^{S_{K}}|x^{S_{K}})\right) \\
				& \ldots \\
		& = \left(\sum_{z^{S_{1}}}  \hat{P}_{_{S_{1}}}(z^{S_{1}}|x^{S_{1}})\right) \ldots \left(\sum_{z^{S_{K}}}  \hat{P}_{_{S_K}}(z^{S_{K}}|x^{S_{K}})\right)\\
		& = \prod_{S \in M} \sum_{z^{S}}  \hat{P}_{_{S}}(z^{S}|x^{S}) \\
		& = \prod_{S \in M} \mathcal{R}(|S|, |\mathscr{Y}|),
\end{split}
\end{equation}
which completes the proof.
\end{proof}

\section*{Proof of Proposition 2}
\begin{proposition}
Assume $\ruleset$ contains $K$ rules in total, including the else rule, and we have $n$ instances. Then $
\log \left(\prod_{S \in \ruleset} \mathcal{R}(|S|, |\mathscr{Y}|)\right) = \frac{K(|\mathscr{Y}| - 1)}{2} \log n + \mathcal{O}(1)$, where $\mathcal{O}(1)$ is bounded by a constant w.r.t.\ to $n$.
\end{proposition}

\begin{proof}
	The proof directly follows from Theorem~3 of~\cite{silander2008factorized}. Firstly, it has been proven that $\log \mathcal{R}(|S|, |\mathscr{Y}|) = \frac{|\mathscr{Y}| - 1}{2} \log |S| + \mathcal{O}(1)$~\cite{rissanen1996fisher}. Next, under the mild assumption that $|S|$ grows linearly as the full sample size $n$, we have $\log |S| = \log ((\gamma + o(1))n) = \log n + \mathcal{O}(1)$. Hence, $\log \prod_{S \in M} \mathcal{R}(|S|, |\mathscr{Y}|) = \sum_{S}\log \mathcal{R}(|S|, |\mathscr{Y}|)$ $= \frac{K(|\mathscr{Y}| - 1)}{2} \log n + \mathcal{O}(1)$, which completes the proof. 
\end{proof}
